# Supplementary material for: SteelHuman: Predicting Operator Estimates of Steel-Scrap Composition from Sparse RGB Views
Source: arXiv:2611.04317 source file (2026-11-03)
Supplement: Supplementary file 2 [file supplementary_preamble.tex]

\usepackage{amsmath}
\usepackage{amssymb}
\usepackage{booktabs}
\usepackage{float}
\usepackage{graphicx}
\usepackage{microtype}
\usepackage{placeins}
\usepackage{tabularx}

\renewcommand{\thesection}{\Alph{section}}
\renewcommand{\thesubsection}{\thesection.\arabic{subsection}}
\renewcommand{\thefigure}{S\arabic{figure}}
\renewcommand{\thetable}{S\arabic{table}}
\renewcommand{\theequation}{S\arabic{equation}}

\newcommand{\TV}{\operatorname{TV}}
\newcommand{\figref}[1]{Fig.~\ref{#1}}
\newcommand{\tabref}[1]{Table~\ref{#1}}
\newcommand{\secref}[1]{Sec.~\ref{#1}}

\newcommand{\suppplaceholder}[2]{%
  \fbox{%
    \begin{minipage}[c][#1][c]{0.94\linewidth}
      \centering\small\itshape #2
    \end{minipage}%
  }%
}
